# Supplementary material for: Neural Generation Meets Real People: Building a Social, Informative Open-Domain Dialogue Agent
Source: arXiv:2207.12021 source file (2023-01-17)
Supplement: Supplementary file 1 [file infilling.tex]

Below, we describe more details as to template-based infilling.

\subsection{Methods}

Let $\mathcal{E}$ be some entity. We want to generate topical sentences from a set of templates $t_1, \ldots, t_n$ from knowledge about this entity, which we have as statements $\{ k(\mathcal{E})^{(1)}, \ldots, k(\mathcal{E})^{(n)} \}$. We generate a grounded statement via the following steps:

\begin{itemize}
    \item \textbf{Knowledge retrieval}: we retrieve a set of statements $k_1, k_2, k_3, \ldots$ and match them to templates $t_1, t_2, t_3, \ldots$ based on some criterion of relevancy/topicality. Currently, this is done via a vector similarity-based search.
    \item \textbf{Infilling}: For each template/knowledge pair $(t_i, k_i)$, we generate a \textbf{completion} $c_i$, which is a possible full response.
    \item \textbf{Reranking}: The set of completions is reranked using several criteria, depending on the use case. The response is then returned as the final output. 
\end{itemize}

Importantly, each of these steps can be performed without significant training on a large dataset. 
We were able to train our infilling model with only $\sim 4286$ manually-curated and GPT-generated examples.

\subsection{Knowledge retrieval}

In this step, given a large amount of information (e.g. from Wikipedia), we want to retrieve a certain amount of \textit{condensed} information that (a) fits in the context window of the infilling model and (b) relates to the templates that we have on hand for the current entity.  
Given an entity brought up by the user, we first retrieve the set of possible templates by matching the entity's WikiData categories against a pre-written set of templates.
We then bucket the total knowledge into windows of $W$ sentences (in our experiments, we use $W = 3$). 
For each window, we compute the sentence embedding using the method of \citet{arora2016simple}.
We then compute the pairwise dot product similarity between window embeddings and template embeddings.
Finally, the top $k$ (template, knowledge) pairs are used as input to the infilling phase.

\subsection{Template embedding generation}

We experiment with various methods for template embedding generation.
We first used \citet{arora2016simple}'s method to generate an embedding directly from the template; however, this resulted in poor results due to domain shift. 
Instead, a more effective strategy was to provide a set of fuzzy keywords for each template.
For example, for the template

\vspace{5pt}

\fbox{``[city]'s most famous landmark is [thing].''}

\vspace{5pt}

we annotate the following keywords: 
\textit{\{``city'', ``landmark'', ``visit'', ``site'', ``tourist''\}}.
To calculate the similarity between a knowledge embedding and the template, we then calculate the pairwise similarity between the knowledge embedding and each keyword, taking the mean of the top $K$ similarities; this allows for multimodality in the use of a template.

This approach is a quick-and-dirty solution: it can easily be done intuitively by human annotators in a limited amount of time, and allows for simple retrieval that usually succeeds. 
However, it is inflexible; in our preliminary quantitative results, we found that it prioritizes areas with high knowledge density over those that are more interesting and novel.
We discuss considerations for future models in our Discussion.

\subsection{Knowledge selection}

In the setting of an Alexa Prize socialbot, our infilling algorithm can draw knowledge from any source; in our implementation, we rely on Wikipedia.
However, Wikipedia articles, especially those for popular entities, can be very long.
This can lead to two problems:
\begin{itemize}
    \item The knowledge retrieved may be very specific. For example, when discussing \textit{Italy}, the retrieval model is likely to retrieve information about specific Renaissance-era artists for the \textit{culture} template.
    \item The knowledge retrieved may be irrelevant to the current subject of discussion. If the model retrieves an arbitrary template every turn, this usually leads to a disjointed and confusing conversation in a multi-turn dialogue setting.
\end{itemize}

To solve this, we only retrieve from a particular Wikipedia \textit{section} at a time. 
During the first turn of the conversation, we retrieve from the intro section if it exists in our datastore; this allows us to make general statements, at the cost of specificity.
On the next turn, we select the section with the highest TF-IDF overlap with the user utterance; this allows for some level of topical `acknowledgement' of the user utterance.

\subsection{Neural Infilling}

In this step, given a textual context and a template, we want to generate an infilled version of the template.
To do so, we apply a fine-tuned BART model \cite{lewis2020bart}. As input, we provide the context and template separated by a \texttt{[SEP]} token; for example, for the above example, we would provide:

``I love \tm{entity} because of \tm{his/her} album \tm{album}, which \mask. {\color{orange} \textsf{\textbf{[SEP]}}} ``Adele Laurie Blue Adkins MBE is an English singer-songwriter. In 2007, she received the Brit Awards Critics' Choice Award and won the BBC Sound of 2008 poll. Her debut album, 19, was released in 2008. It is certified 8× platinum in the UK and triple platinum in the US. {\color{orange} \textsf{\textbf{[SEP]}}}'' 

The model is then trained to predict the entire infilled template. This is largely a copying operation; for example, in the above example, the tokens ``I love \ldots because of \ldots album \ldots which \ldots .'' can be copied directly from the input.

\paragraph{Infilling} We note that the infilling procedure is very similar to the denoising operation of a masked language model \citep{devlin2018bert, ghazvininejad2019mask}. 
However, since we use a \texttt{seq2seq} language model, we can generate arbitrarily large numbers of tokens per position, allowing for more flexible generations; for example, we are able to generate ``\maskr{was released in 2008}'' from a single \texttt{\mask} token, something that wouldn't be possible without Gibbs sampling-style decoding \citep{wang2019bert, salazar2019masked}; additionally, it is possible to not infill a slot at all.

\paragraph{Dataset} 
We generate $\sim4143$ training pairs using GPT-3 \citep{brown2020language}, a large pretrained generative language model capable of few-shot contextual learning.
First, we take utterances from the Topical Chat dataset \citep{gopalakrishnan2019topical}, a dataset of human conversations grounded in Wikipedia entities.
We match the utterances to Wikipedia paragraphs using TF-IDF similarity score, taking only paragraph-entity pairs with TF-IDF similarity between 0.04 and 0.08.

For each utterance, we generate two templates using the few-shot priming in Table \ref{tab:priming}, only keeping distinct and non-erroneous templates (i.e. the number of generated infills equals the number of slots in the template).
Since the task is relatively deterministic, we use a temperature of $0.3$.
During training, the model is then trained to infill the template back to the original utterance, conditioned on the Wikipedia paragraph.

\begin{table*}
    \centering
    \begin{adjustbox}{max width=\textwidth}
    \begin{tabular}{@{}lll@{}}

Email and file sharing are very useful Internet services that I use daily. & [Product] is a very useful service that I use [time]. & Email and file sharing ;; daily \\
Do you know what the New Zealand basketball team is called? & Do you know what the [location] [sport] team is called? & New Zealand ;; basketball \\
I'm a really big fan of the Beatles. I especially love their song Penny Lane. & I'm a really big fan of [band]. I especially love their song [song]. & The Beatles ;; Penny Lane \\
Superman is a fictional superhero, me also like batman and spider-man. & [Character] is a fictional [occupation], I also like [character]. & Superman ;; superhero ;; batman and spider-man \\
Computers do so much now, not just the original use as a calculating device. &  Computers do so much now, not just the original use as a [purpose]. & calculating device \\
I'm a big fan of Napoleon. & I'm a big fan of [person]. & Napoleon \\

    \end{tabular}
    \end{adjustbox}

    \vspace*{1ex}

    \caption{The few-shot priming that we use to generate templates using GPT-3.}
    \label{tab:priming}
\end{table*}

\paragraph{Manual data augmentation}
Although generating data this way is easy, we find that it suffers from domain shift. Despite the fact that our priming sentences mostly have several slots, as do the templates we use in practice, most of the templates (94.3\%) generated by GPT-3 only have one slot; all but 3 of the remainder only have two slots.
The reason for this shift is unclear.

To ameliorate this issue, we manually augment the data with multiple hand-written examples drawn from the Wizard of Wikipedia dataset \citep{dinan2018wizard}.
Since most utterances in this dataset simply rephrase the original knowledge statement, we create our own utterances which are more similar to the templates we use in practice. We create $143$ of these examples, fine-tuning our model on both the handwritten examples and the GPT-3 examples without any weighting.

\paragraph{The \mask token} By convention, we use \tm{bracketed words} to represent single-word slots; we use the \mask token to represent a larger amount of text to be copied from the input. We draw this directly from BART training, which uses \mask to represent a multi-word denoising objective. Since there are no \mask tokens in our GPT-3-generated dataset, we manually write templates involving \mask as part of our $143$ examples. (Note: one can use BART to infill slots in templates zero-shot due to this denoising objective, but our preliminary experiments suggested that this was typically unsuccessful due to being trivial/uninteresting infills.)

\subsubsection{Implementation details}

\paragraph{Fine-tuning} We fine-tune the BART-base model (139M parameters) on the set of $4286$ examples generated using GPT-3 using the Adam optimizer \citep{kingma2014adam} with learning rate $1\text{e}-5$ and otherwise default parameters. We use the HuggingFace reimplementation for all models. We do no validation due to limited data, stopping after 3 epochs to avoid overfitting.

\paragraph{Decoding} We decode using beam search with beam size $ = 2$. Empirically, we found that using greedy search (beam size $= 1$) can lead to failure to copy correctly due to high-probability, incorrect subwords being copied.

\subsection{Reranking}

Once the infiller has finished, we have a set of possibly topical utterances generated based on knowledge about the current entity. We now need to select a coherent, interesting response that is related to the user's previous subject of conversation. To do so, we calculate the mean per-token negative log-likelihood of each statement using a GPT-2 medium model fine-tuned on the EmpatheticDialogues dataset \citep{rashkin2018towards}, as well as its absolute score using the DialoGPT \texttt{updown} reranking model \citep{zhang2019dialogpt}, which is trained on upvote/downvote data from Reddit. We then rerank using the following formula:
\begin{align*}
    \text{score} = \text{score}_\text{DialoGPT} - 0.25 \times \text{NLL}_\text{GPT}.
\end{align*}
where the DialoGPT score is a probability between 0-1 and the NLL tends to be around $-2$.
Although this is not entirely mathematically sound (adding what is \textit{technically} a probability and a log-likelihood), it seems to work well in practice.
Specifically, the DialoGPT reranking score seems to select for interesting utterances with novel information, while the GPT likelihood seems to select for fluency (rather than numerous noun phrases put together).

\subsection{Results}

We find that our method achieves good qualitative results; however, we defer human evaluation to future updates.

Here are some examples:

\begin{itemize}
\item Template: I love [song] because of its [quality].
Infill:  I love "Someone Like You" because of its beautiful lyrics.
\item Template: The best qualities of [singer]'s voice are \mask.
Infill:  The best qualities of Adele's voice are its power and range.
\item Template: [singer] has won awards such as \mask for her songs.
Infill:  Adele has won awards such as a Grammy and an Academy Award for her songs.
\item Template: I still remember [year], when it seemed like [song] was on every [genre] station.
Infill:  I still remember 2009, when it seemed like Adele's "Chasing Pavements" was on every pop station.
\item Template: I really like [artist] because she is so [adjective].
Infill:  I really like Adele because she is so critically acclaimed.
\item Template: My favorite album by [artist] is [album] because it's so [adjective]. \mask
Infill:  My favorite album by Adele is 21 because it's so critically acclaimed. It's won six Grammys and an Academy Award.
\item Template: I've been following her since she first started [action] at [place]
Infill:  I've been following her since she first started performing at the Bluebird Cafe in Nashville.
\item Template: Do you remember when \mask?
Infill:  Do you remember when Adele won a Grammy for 21?
\item Template: I hear that [group] released the album [name].
Infill:  I hear that Adele released the album 25.
\end{itemize}
